# Supplementary material for: Azetidinium as Cation in Lead Mixed Halide Perovskite Nanocrystals of Optoelectronic Quality
Source: arXiv:1905.09073 ancillary file (2019-05-22)
Supplement: Supplementary file 1 [file Supplementary_Info.pdf]

# Supplementary Information: Azetidinium as Cation in Lead Mixed Halide Perovskite Nanocrystals of Optoelectronic Quality

Sameer Vajjala Kesava,[1] Yasser Hassan,[1] Alberto Privitera,[1]
Aakash Varambhia,[2] Henry J. Snaith,[1] and Moritz K. Riede[1]

[1]*Department of Physics, University of Oxford, OX1 3PU, England, UK*

[2]*Department of Materials, University of Oxford, OX2 6HT, England, UK*

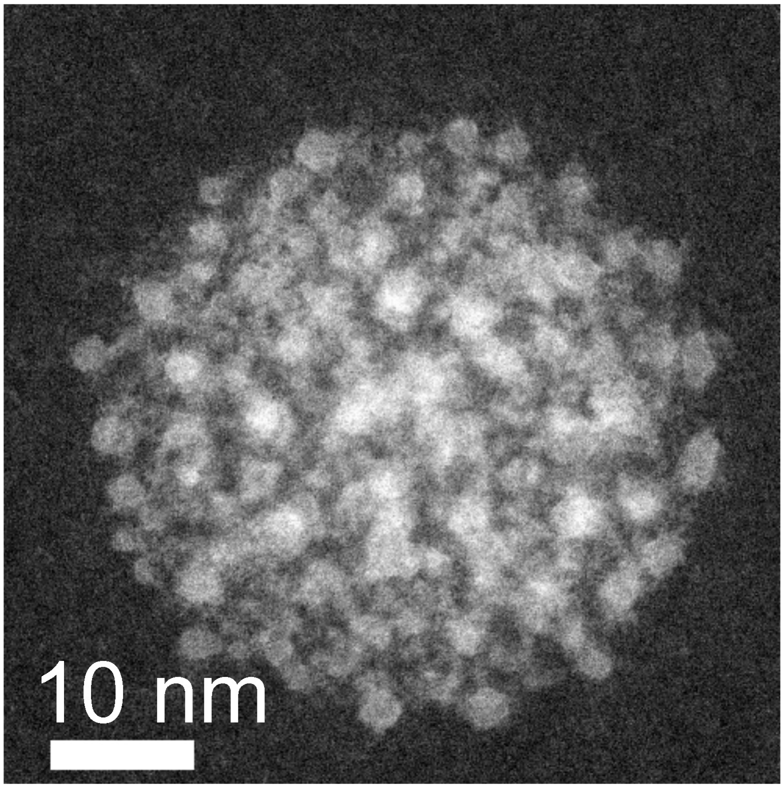


FIG. S1. TEM image of the ensemble of nanocrsytals scanned for EDS spectroscopy. The obtained spectra (in main text, Figure 4) verified the presence of Cl along with Pb and I.

TABLE S1. Table shows elemental compositions and corresponding X-ray counting statistics errors calculated from EDS spectra in Figure 4 obtained from the nanocrystal ensemble in Figure S1. In addition to the counting errors, the compositions could have large systematic errors upto 20% due to use of inbuilt k-factor routines [1, 2]. Moreover, errors could arise from using a combination of K+L lines for the k-factor quantification due to the different ionisation mechanism for each line, further adding to the uncertainty in estimating the atomic ratios. Hence, the true composition, and thus the stoichiometry, of our perovskite could not be accurately determined.

| **Element** | **Atomic Percent** | **Counting Statistics Error ±%** |
|---|---|---|
| Pb | 47 | 7.3 |
| I | 39 | 4.8 |
| Cl | 14 | 6.6 |

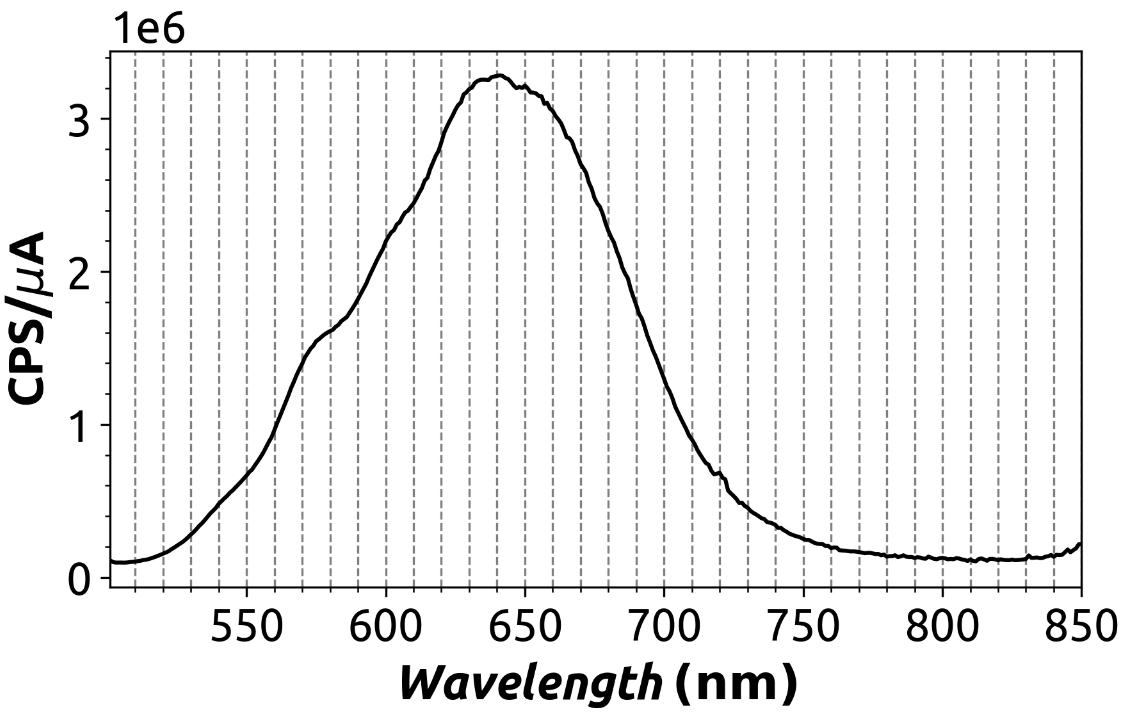


FIG. S2. Steady-state photoluminescence data of the unfiltered and dried $AzPbI_2Cl$ colloids. Excitation wavelength is 450 nm.

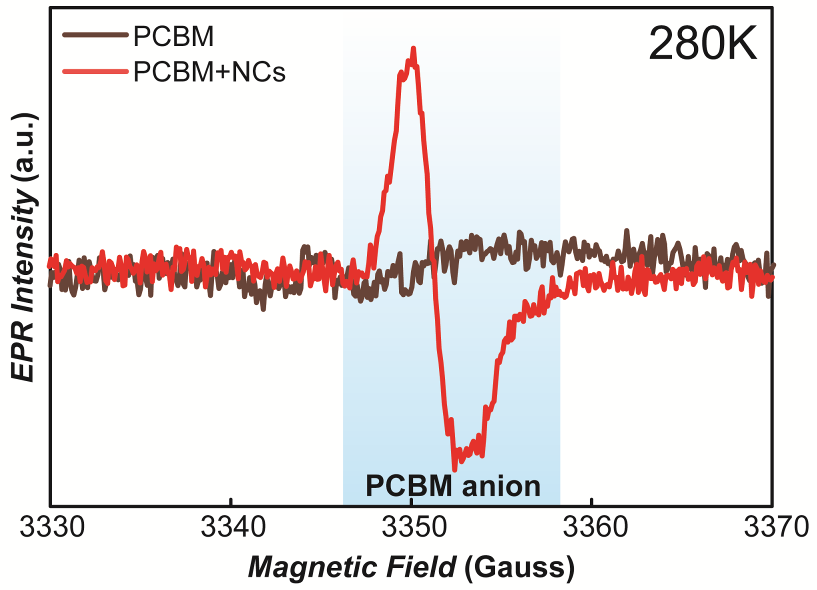


FIG. S3. LEPR spectra of PCBM (brown) and PCBM:NCs blend (red) films acquired at 280 K.

[1] K. E. MacArthur, T. J. A. Slater, S. J. Haigh, D. Ozkaya, P. D. Nellist, and S. Lozano-Perez, Microscopy and Microanalysis **22**, 7181 (2016).

[2] M. Watanabe, Z. Horita, and M. Nemoto, Ultramicroscopy **65**, 187 (1996).
